# Supplementary material for: On the Separability Problem of VASS Reachability Languages
Source: arXiv:2401.16095 source file (2026-11-16)
Supplement: Supplementary file 1 [file appendix.tex]

\appendix
\section{Appendix: DMGTS}
\begin{proof}[Proof of Lemma~\ref{Lemma:EasyInclusion}]
    Let $\aword\in\rightlangof{\admgts}$.
    Then there is a run $\arun$ in~$\admgts$ labeled by $\edgelabelof{\apath}=\aword$ that remains non-negative and that is accepting on $\rightside$. 
    By the definition of DMGTS, the effects of letters on the counters in $\rightside$ agree with the effects that these letters have in the VASS $\dyckvas_{\dyckdims}$.
    This allows us to construct a run $\apath'\in\acceptof{\nat}{\omegaleq}{\dyckvas_{\dyckdims}}$ that has the same counter valuations and updates. 
    Hence, we have $\aword\in \dycklangn{\dyckdims}$. 
\end{proof}
\section{Appendix: The Decomposition}

In this section, we provide the missing proofs from Section~\ref{Section:OurDecomposition}, followed by the analysis of the complexity of the algorithm from the proof of Lemma~\ref{Lemma:DecoupledDecomposition}.
We preface the missing proofs with the adapting the Rackoff-styled observations in \cite{Leroux19} to our needs.

As we mention in the main paper, our decomposition is based on the decomposition by Leroux et al. in \cite{Leroux19}.
For this reason, many proofs we feature are adaptations of the ones in \cite{Leroux19}.
Because our setting differs from that of \cite{Leroux19} non-trivially, we adapt the proofs to our setting instead of using them as black-boxes.
The biggest difference is this.
DMGTS define two languages, one per counter set $\leftside$ and $\rightside$, where the language associated with one side does not track the constraints on the other side.
Additionally, we need the faithfulness invariant, which is not needed in \cite{Leroux19}.

\subsection{Preliminary Proofs}

As alluded to, we first show the following observation which is an adaptation of Lemma A.1 from the appendix of \cite{Leroux19}.
For a set of counters $\countersp$ our version of the observation states the following.
If we have an integer run, where each counter (i) exceeds some doubly exponential bound in $C$, the number of counters $d$, and the largest effect of a transition $l$ along the run and (ii) remains positive until this happens, then there is an $\countersp$-run that reaches a value that covers $C$ in all counters $i\in\countersp$.
Our version of the observation differs from the one used in \cite[Lemma A.1]{Leroux19}, in that we allow counters to become negative after exceeding the bound.
We recall the proof

\begin{lem}\label{Lemma:RackoffesqueAppendix}
    Let $\precovering$ be a precovering graph with the largest transition effect $l$, $C\geq 2$, $\countersp\subseteq\leftside\cup\rightside$, and $\apath\in\pathsof{\ints}{\precovering}$ 
    with $$\apath=(\astate_{0}, \aconf_{0})\anedge_{0}\ldots\anedge_{k-1}(\astate_{k}, \aconf_{k}).$$
    If for all $\aplace\in\countersp$, there is an $i\leq k$ with $\coordacc{\aconf_{i}}{\aplace}\geq(\sizeof{\nodesof{\precovering}}\cdot l\cdot C)^{\sizeof{\countersp}+1!}$, and $\coordacc{\aconf_{i'}}{\aplace}\geq 0$ for all $i'\leq i$, then there is a run $\apathp\in\pathsof{\countersp}{\precovering}$ of size at most $(\sizeof{\nodesof{\precovering}}\cdot l\cdot C)^{\sizeof{\countersp}+1!}$ where $\coordacc{\apathp}{\lastindex}=(\astate_{k}, \aconf)$, $\coordacc{\apathp}{\firstindex}=(\astate_{0}, \aconf_{0})$, and $\coordacc{\aconf}{\aplace}\geq C$ for all $\aplace\in\countersp$.
\end{lem}

\begin{proof}[Proof of Lemma~\ref{Lemma:Rackoffesque}]
    Let $\precovering$, $\countersp$, $\apath$, and $l$ be defined as stated in the premise of the lemma, and $\apath$ additionally the shortest run with this property.
    First, we define $\alpha_{i}$ for $i\leq\sizeof{\leftside\cup\rightside}$ inductively.
    We define $\alpha_{0}=\sizeof{\nodesof{\precovering}}$, and $\alpha_{i}=\sizeof{\nodesof{\precovering}}\cdot(l\cdot \alpha_{i-1} + C)^{i} + \alpha_{i-1}$ for $i>1$.
    Over approximating, we get 
    $$\alpha_{i}\leq \sizeof{\nodesof{\precovering}}\cdot(l\cdot \alpha_{i-1}\cdot C)^{i}+\alpha_{i-1}\leq(\sizeof{\nodesof{\precovering}} \cdot l\cdot \alpha_{i-1}\cdot C)^{i+1}.$$
    We can apply the inductive definition to get 
    $$\alpha_{i}\leq (\sizeof{\nodesof{\precovering}}\cdot l\cdot C)^{i+1!}$$

    Our proof is by induction on $\sizeof{\countersp}$.
    For the base case, we take $\countersp=\emptyset$.
    Then, both the premise and the requirements become trivial.
    Since there is a run $\apath$ that starts from $\astate_{0}$ and ends at $\astate_{k}$, we can find a run of size at most $\sizeof{\nodesof{\precovering}}=\alpha_{0}$ between these nodes.
    
    For the inductive case, let Lemma~\ref{Lemma:Rackoffesque} hold for all $\countersp'\subset\countersp$.
    The premise of the lemma gives us $i_{\aplace}\leq k$ for each $\aplace\in \countersp$ where $\coordacc{\aconf_{i_{\aplace}}}{\aplace}\geq \alpha_{\sizeof{\countersp}}\geq l\cdot \alpha_{\sizeof{\countersp}-1} + C$ and $\coordacc{\aconf_{i'}}{\aplace}\geq 0$ for all $i'\leq i_{\aplace}$.
    Wlog. assume $i_{\aplace}$ to be minimal for each $\aplace\in\countersp$.
    Let $\countersp'$ be the set of counters $\aplace$ that minimize $i_{\aplace}$.
    Fix some $\aplace\in\countersp'$.
    The remainder of the run $(\astate_{i_{\aplace}}, \aconf_{i_{\aplace}})\ldots(\astate_{k}, \aconf_{k})$ satisfies the premise of the lemma for $\countersp\setminus\countersp'$.
    Since $i_{\aplace}$ is minimal and $\apath$ is a $\countersp$-run, we know that for all $\aplace\in\countersp$ and $i'<i_{\aplace}$, $\coordacc{\aconf_{i'}}{\aplace}<l\cdot \alpha_{\sizeof{\countersp}-1}+C$.
    Then, each counter in $\countersp$ can have at most $l\cdot \alpha_{\sizeof{\countersp}-1}+C$ different values.
    We have $i_{\aplace}<\sizeof{\nodesof{\precovering}}\cdot(l\cdot\alpha_{\sizeof{\countersp}-1} + C)^{\sizeof{\countersp}}$ since  $\apath$ is minimal and we could eliminate a loop from $\apath$ if this were to not hold. 
    Denote the run up to this point as $\apath_{0}$.
    Observe that the remaining run $(\astate_{i_{\aplace}}, \aconf_{i_{\aplace}})\ldots(\astate_{k}, \aconf_{k})$ fulfills the premise of the lemma for the counters $\countersp\setminus\countersp'$:
    for all $n\in\countersp\setminus\countersp'$, we know that there is a $i_{\aplace} < i_{m}\leq k$ where $\coordacc{\aconf_{i_m}}{m}\geq \alpha_{\sizeof{\countersp}}(C)\geq \alpha_{\sizeof{\countersp\setminus\countersp'}}(C)$ and $\coordacc{\aconf_{i'}}{m}\geq 0$ for all $i'\leq i_{m}$.
    Then the induction hypothesis applies to show that there is a $\countersp\setminus\countersp'$-run $\apathp_{1}$ from $(\astate_{i_{\aplace}}, \aconf_{i_{\aplace}})$ of length at most $\alpha_{\sizeof{\countersp\setminus\countersp'}}(C)$ that reaches $(\astate_{k}, \aconf)$ with $\coordacc{\aconf}{\aplace}\geq C$ for all $m\in\countersp\setminus\countersp'$.
    Let $\apathp=\ldots(\astate_{k}, \aconf)$ be the run  obtained by following up $\apath_{0}$ by $\apathp_{1}$.
    We claim that $\apathp$ is a $\countersp$-run with $\coordacc{\aconf}{n}\geq C$.
    This is already clear for all $n\in\countersp\setminus\countersp'$.
    For $n\in\countersp'$, we observe that $\apath_{0}$ is by definition positive on these counters, and $\coordacc{\aconf_{i_n}}{n}\geq l\cdot \alpha_{\sizeof{\countersp}-1}+C \geq l\cdot \alpha_{\sizeof{\countersp\setminus\countersp'}}+C$.
    Then, since $\apathp$ takes at most $\alpha_{\sizeof{\countersp\setminus\countersp'}}$ transitions, the counter $n$ remains above $C\geq 0$ for all prefixes of $\apathp_{1}$.
    This concludes the proof.
\end{proof}

We now show Lemma~\ref{Lemma:ConsistentSpec}.
We break down its conclusions into two proofs, one for the implied inclusion and one for the implied faithfulness.
In the following proofs, we write $\admgts_{0}\consspec\admgts_{1}$ mean that $\admgts_{0}$ is a consistent specialization of $\admgts_{1}$.
We also write $(p, c).c$ for a configuration $(p, c)$ to denote the counter valuation of the configuration.

\begin{proof}[Proof Sketch of Lemma~\ref{Lemma:ConsistentSpec}, Inclusion]
    The proof is by structural induction over the proof tree for $\consspec$.
    By this we refer to a tree labeled by pairs of DMGTS $(\admgts_{0}, \admgts_{1})$ where (i) the node is a leaf where the properties (1) and (2) have been applied to show $\admgts_{0}\consspec\admgts_{1}$ or (ii) the node is not a leaf and the inductive case is used to show $\admgts_{0}\consspec\admgts_{1}$ by inserting the relation shown in its successor into a context.
    Our inductive invariant is stronger than the conclusion of Lemma~\ref{Lemma:ConsistentSpec}: If $\admgts_{0}\consspec\admgts_{1}$, then for all $\apath\in\interacceptofshort{\leftside}{\admgts_{0}}$, there is a $\apathp\in\interacceptofshort{\leftside}{\admgts_{1}}$ with $\apath\pathequiv\apathp$.
    Because $\pathequiv$ preserves labels, this clearly implies the desired inclusion.
    For the base case, we have $\admgts_{1}=(\precovering, \mu)$ for some precovering graph $\precovering$, where (1) and (2) hold to show $\admgts_{0}\consspec\admgts_{1}$.
    Let $\apath\in\interacceptofshort{\leftside}{\admgts_{0}}$.
    We know $\coordacc{\coordacc{\apath}{\firstindex}.\aconf}{\leftside} \omegaleq\coordacc{\inmarkingof{\admgts_{0}}}{\leftside}$, $\coordacc{\coordacc{\apath}{\lastindex}.\aconf}{\leftside}\omegaleq\coordacc{\coordacc{\outmarkingof{\admgts_{0}}}{\leftside}$, $\coordacc{\apath}{\firstindex}.\aconf}{\rightside} \omegalequiv{\charmod}\coordacc{\inmarkingof{\admgts_{0}}}{\rightside}$, and $\coordacc{\coordacc{\apath}{\lastindex}.\aconf}{\rightside}\omegalequiv{\charmod}\coordacc{\outmarkingof{\admgts_{0}}}{\rightside}$.
    The second part of (1) tells us that there is a $\apathp\in\pathsof{\ints}{\admgts_{1}}$ with $\apathp\pathequiv\apath$.
    The relation $\pathequiv$ keeps the counter valuations intact.
    So positivity on $\leftside$ counters is kept, and the constraints are kept: 
    \begin{align*}
        \coordacc{\coordacc{\apathp}{\firstindex}.\aconf}{\leftside}&\omegaleq\coordacc{\inmarkingof{\admgts_{0}}}{\leftside}\omegaleq\coordacc{\inmarkingof{\admgts_{1}}}{\leftside}\\
        \coordacc{\coordacc{\apathp}{\lastindex}.\aconf}{\leftside}&\omegaleq\coordacc{\outmarkingof{\admgts_{0}}}{\leftside}\omegaleq\coordacc{\outmarkingof{\admgts_{1}}}{\leftside}\\
        \coordacc{\coordacc{\apathp}{\firstindex}.\aconf}{\rightside}&\omegalequiv{\charmod}\coordacc{\inmarkingof{\admgts_{0}}}{\rightside}\omegaleq\coordacc{\inmarkingof{\admgts_{1}}}{\rightside}\\
        \coordacc{\coordacc{\apathp}{\lastindex}.\aconf}{\rightside}&\omegalequiv{\charmod}\coordacc{\outmarkingof{\admgts_{0}}}{\rightside}\omegaleq\coordacc{\outmarkingof{\admgts_{1}}}{\rightside}
    \end{align*}
    At each line, the first inequality follows from $\apath\in\interacceptofshort{\leftside}{\admgts_{0}}$, and the fact that $\pathequiv$ keeps the counter valuations intact.
    The second inequality follows from the first part of (1) that constraints the valuations of $\openmgts_{0}$ with respect to $\precovering$.
    For the inductive case, let $\admgts_{i}=\acontext{\admgts_{i}'}$ for some DMGTS $\admgts_{i}'$ for each $i\in\set{0, 1}$, where $\admgts_{0}'\consspec\admgts_{1}'$.
    Let $\apath\in\interacceptofshort{\leftside}{\admgts_{0}}$.
    We break this run down into $\apath=\apath_{0}.\apath_{1}.\apath_{2}$ where $\apath_{1}$ is the part of the run in $\admgts_{0}'$, and $\apath_{0}.\contextvar.\apath_{2}$ the remaining part in the outer context $\acontext{\contextvar}$.
    Compositionality of $\interacceptofshort{\leftside}{-}$ tells us $\apath_{1}\in\interacceptofshort{\leftside}{\admgts_{0}'}$.
    Using the induction hypothesis, we get a run $\apathp_{1}\in\interacceptofshort{\leftside}{\admgts_{1}'}$ with $\apathp_{1}\pathequiv\apath_{1}$.
    Using compositionality and the fact that $\acontext{\contextvar}$ is the same between $\admgts_{0}$ and $\admgts_{1}$, we deduce $\apathp=\apath_{0}.\apathp_{1}.\apath_{2}\in\interacceptofshort{\leftside}{\admgts_{1}}$.
    Since $\apath_{1}\pathequiv\apathp_{1}$, it is clear that $\apath_{0}\pathequiv\apath_{1}$.
    This concludes the proof.
\end{proof}

\begin{proof}[Proof Sketch of Lemma~\ref{Lemma:ConsistentSpec}, Faithfulness]
    We do a structural induction similarly to the proof of Lemma~\ref{Lemma:ConsistentSpec}.
    We maintain two invariants.
    If $\admgts_{0}\consspec\admgts_{1}$, then 
    \begin{itemize}
        \item [(a)] For all $\apath\in\interacceptof{\ints}{\restrictto{\omegalequiv{\charmod}}{\rightside}}{\admgts_{0}}$, there is $\apathp\pathequiv\apath$ with $\apathp\in\interacceptof{\ints}{\restrictto{\omegalequiv{\charmod}}{\rightside}}{\admgts_{1}}$.
        \item [(b)] If $\admgts_{1}$ is faithful, for all runs  $\apath\in\interacceptof{\ints}{\restrictto{\omegalequiv{\charmod}}{\rightside}}{\admgts_{0}}$ with 
        $\coordacc{\coordacc{\apath}{\firstindex}.\aconf}{\rightside}\omegaleq\coordacc{\inmarkingof{\admgts_{1}}}{\rightside}$, 
        and $\coordacc{\coordacc{\apath}{\lastindex}.\aconf}{\rightside}\omegaleq\coordacc{\outmarkingof{\admgts_{1}}}{\rightside}$, we have $\apath\in\interacceptof{\ints}{\rightside}{\admgts_{0}}$.
    \end{itemize}
    We also use the fact that $\inmarkingof{\admgts_{0}}\omegaleq\inmarkingof{\admgts_{1}}$ and $\outmarkingof{\admgts_{0}}\omegaleq\inmarkingof{\admgts_{1}}$, which can be shown by standard induction.
    This fact, applied with (b), shows the implication from the faithfulness of $\admgts_{1}$ to the faithfulness of $\admgts_{0}$, in Lemma~\ref{Lemma:ConsistentSpec}.
    For the base case, let $\admgts_{1}=(\precovering, \charmod)$ 
    for some precovering graph $\precovering$, where (1) and (2) show $\admgts_{0}\consspec\admgts_{1}$.
    Let $\apath\in\interacceptof{\ints}{\restrictto{\omegalequiv{\charmod}}{\rightside}}{\admgts_{0}}$.
    Because of (1), we know that there is a $\apathp\in\pathsof{\ints}{\precovering}$ with $\apathp\pathequiv\apath$.
    Since (1) tells us that $\inmarkingof{\admgts_{0}}$ and $\outmarkingof{\admgts_{0}}$ are stricter than $\inmarkingof{\admgts_{1}}$ and $\outmarkingof{\admgts_{1}}$, and $\precovering$ does not have intermediate valuations, $\apathp\in\interacceptof{\ints}{\restrictto{\omegalequiv{\charmod}}{\rightside}}{\admgts_{1}}$.
    This shows (a).
    Invariant (b) is just (2).
    This concludes the base case.
    For the inductive case, let $\admgts_{0}=\acontext{\admgts_{0}'}$ and $\admgts_{1}=\acontext{\admgts_{1}'}$ with $\admgts_{0}'\consspec\admgts_{1}'$.
    Let $\apath\in\interacceptof{\ints}{\restrictto{\omegalequiv{\charmod}}{\rightside}}{\admgts_{0}}$.
    We have $\apath=\apath_{0}.\apath_{1}.\apath_{2}$ where $\apath_{1}$ is the part of the run in $\admgts_{0}'$, and $\apath_{0}.\contextvar.\apath_{2}$ is the part of the run in the outer context $\acontext{\contextvar}$.
    For (a), we invoke the induction hypothesis on $\apath_{1}$ and use compositionality, same as in the proof of Lemma~\ref{Lemma:ConsistentSpec}, Inclusion.
    For (b), let $\admgts_{1}$ be faithful, let $\apath\in\pathsof{\ints}{\admgts_{0}}$, 
    $\coordacc{\coordacc{\apath}{\firstindex}.\aconf}{\rightside}\omegaleq\coordacc{\inmarkingof{\admgts_{1}}}{\rightside}$, and $\coordacc{\coordacc{\apath}{\lastindex}.\aconf}{\rightside}\omegaleq\coordacc{\outmarkingof{\admgts_{1}}}{\rightside}$ also hold.
    By (a) and compositionality, we obtain 
    $\apathp=\apath_{0}.\apathp_{1}.\apath_{2}\in\interacceptof{\ints}{\restrictto{\omegalequiv{\charmod}}{\rightside}}{\admgts_{1}}$ with $\apathp_{1}\pathequiv\apath_{1}$.
    Since $\pathequiv$ does not change counter valuations, and $\apath$ already reaches the initial and final valuations of $\admgts_{1}$, we know that $\apathp\in\acceptof{\ints}{\rightside}{\admgts_{1}}$.
    Using the faithfulness of $\admgts_{1}$, $\apathp\in\interacceptof{\ints}{\restrictto{\omegalequiv{\charmod}}{\rightside}}{\admgts_{1}}$, and $\apathp\in\acceptof{\ints}{\rightside}{\admgts_{1}}$,  we deduce $\apath\in\interacceptof{\ints}{\rightside}{\admgts_{1}}$.
    This yields $\apathp_{1}\in\interacceptof{\ints}{\rightside}{\admgts_{1}'}$, which implies $\coordacc{\coordacc{\apath_{1}}{\firstindex}.\aconf}{\rightside}\omegaleq\coordacc{\inmarkingof{\admgts_{1}'}}{\rightside}$ and $\coordacc{\coordacc{\apath_{1}}{\lastindex}.\aconf}{\rightside}\omegaleq\coordacc{\outmarkingof{\admgts_{1}'}}{\rightside}$ by the properties of $\pathequiv$.
    We also note that  $\apath\in\interacceptof{\ints}{\restrictto{\omegalequiv{\charmod}}{\rightside}}{\admgts_{0}}$ implies 
    $\apath_{1}\in\interacceptof{\ints}{\restrictto{\omegalequiv{\charmod}}{\rightside}}{\admgts_{0}'}$.
    We use induction hypothesis (b) to get $\apath_{1}\in\interacceptof{\ints}{\rightside}{\admgts_{0}'}$. 
    Since the outer run $\apathn{0}.\contextvar.\apathn{2}$ fulfills the remaining requirements by $\sigma=\apath_{0}.\apathp_{1}.\apath_{2}\in\interacceptof{\ints}{\rightside}{\admgts_{1}}$, we get $\apath=\apath_{0}.\apath_{1}.\apath_{2}\in\interacceptof{\ints}{\rightside}{\admgts_{0}}$.
\end{proof}

\subsection{Decomposition Steps}

In this section, we prove Lemma~\ref{Lemma:EdgeDecomposition} and Lemma~\ref{Lemma:CoveringDecomposition}.
They both involve decomposing a precovering graph $(\precovering, \charmod)$ into sets of DMGTS $U$ and $V$ that track extra information.
We do this by enriching the structure of the precovering graph.
To make this enrichment formal and our handling uniform, we define \emph{observer NFA}.
An observer NFA $\anobserver=(\states, \initstates, \edgesof{\precovering}, \transitions, \finalstates)$ for $\precovering$ is an NFA that has the edges $\edgesof{\precovering}$ as its alphabet.
We note that the language of an observer $\langof{\anobserver}\subseteq\edgesof{\precovering}^{*}$ consists of sequences of edges in $\precovering$.
By constructing the product of an observer and a precovering graph, we get a larger automaton that accepts the edge sequences of runs based on the information we want to track. 
We then decompose this automaton into MGTS, in accordance with the valuations of $\precovering$.

\begin{comment}
    A backward consistent assignment is defined symmetrically by changing the direction of the transitions and switching (i) to $\outmarkingof{\precovering}\omegaleq\fbconsistentof{\astate}$ for all $\astate\in\finalstates_{\adfa}$.
    %
    A forward/backward consistent assignment is meant to further specialize the consistent assignment in $\precovering$.
    %
    First condition makes sure that the initial marking of $\precovering$ is respected by the runs in $\adfa$.
    %
    The second condition says that if the assignment stops tracking a counter along a run, than it cannot be tracked again.
    %
    Finally, the last condition guarantees that the consistent assignment of $\precovering$ cannot conflict with the assignment $\fbconsistent$ on any state.
\end{comment}

We define the product $\precovering\times\anobserver$ between an observer $\anobserver=(\states, \initstates, \edgesof{\precovering}, \transitions, \finalstates)$ and a precovering graph $\precovering$ to be the observer $(\nodesof{\precovering}\times\states, \set{\precovering.\groot}\times\initstates, \edgesof{\precovering}, \transitions_{\times}, \set{\precovering.\groot}\times\finalstates)$, where 
\begin{align*}
    \transitions_{\times}=\set{((\astate_0, \astate_1), &\anedge,(\astatep_0, \astatep_1))\mid \\ 
    &\anedge\in\edgesof{\precovering}, \anedge=(\astate_0, \aletter, x, \astatep_0), (\astate_1, \anedge, \astatep_1)\in\transitions}.
\end{align*}
Intuitively, $\precovering\times\anobserver$ simulates $\anobserver$ along the edges $\precovering$ can take during a run.
We construct MGTS along the runs in $\precovering\times\anobserver$.
Towards this construction, we define the precovering graphs.
For each state $\astate$ of $\anobserver\times\precovering$, we define the precovering graph 
\begin{align*}
    \precovering_{\astate}^{\anobserver}&=(\avas_{\astate}^{\anobserver}, (\astate, \precovering.\bal_{\times}(\astate)), (\astate, \precovering.\bal_{\times}(\astate)), \bal_{\times})\\
    \avas_{\astate}^{\anobserver}&=(\sccof{\astate}, \dyckalphn{\dyckdims}, \leftside\cup\rightside, \edges_{\astate}^{\anobserver})
\end{align*}
where $\sccof{\astate}$ is the strongly connected component of $\astate$ in $\precovering\times\anobserver$, and $E_{\astate}^{\anobserver}$ is the set of edges $(\astatep, \aletter, x, \astatep')$ for which $\astatep, \astatep'\in\sccof{\astate}$, $(\astatep, \anedge, \astatep')\in\transitions_{\times}$ hold for some $\anedge=(\astatepp, \aletter, x, \astateppp)\in\edgesof{\precovering}$, and $\precovering.\bal_{\times}(\astate, \astatep)=\precovering.\bal(\astate)$ for $(\astate, \astatep)\in\nodesof{\precovering}\times\states$.
We define the MGTS 
$$\observedmgts{\anobserver}{\apath, \mathsf{raw}}=\precovering_{\astate_{0}}^{\anobserver}.\anupdate_{0}\ldots\anupdate_{k-1}.\precovering_{\astate_{k}}^{\anobserver}$$
for each accepted run $\apath=\astate_{0}.(\astate_{0}, \anedge_{0}, \astate_{1})\ldots (\astate_{k-1}, \anedge_{k-1}, \astate_{k}).\astate_{k}$ in $\precovering\times\anobserver$, where $\anupdate_{i}=(\aletter, x)$ and $\anedge_{i}=(\astatepp, \aletter, x, \astateppp)$ for all $i\leq k-1$.
To keep the valuations of $\precovering$ and $\observedmgts{\anobserver}{\apath}$ coherent, we define the MGTS $\observedmgts{\anobserver}{\apath}$, which is obtained from $\observedmgts{\anobserver}{\apath, \mathsf{raw}}$ by modifying the initial valuation, and the final valuation so that $\inmarkingof{\observedmgts{\anobserver}{\apath}}=\inmarkingof{\precovering}$ and $\outmarkingof{\observedmgts{\anobserver}{\apath}}=\outmarkingof{\precovering}$ hold.
Note that this modification is compatible with the consistent assignments of the first and the last precovering graphs of $\observedmgts{\anobserver}{\apath}$. 
This is a consequence of the definition.

The set of accepted runs in $\precovering\times\anobserver$ is not a finite set.
Since we need a finite set for our decomposition, we define $\basicacceptof{\precovering\times\anobserver}$ to be the set of accepted runs in $\precovering\times\anobserver$ that go from the initial states to the final states without repeating a state.
We are now ready to define the general form of our decompositions.
We write 
$$\decompalongof{\precovering, \charmod, \anobserver}=\setcond{(\observedmgts{\anobserver}{\apath}, \charmod)}{\apath\in\basicacceptof{\precovering\times\anobserver}}.$$

The form of the decomposition gives us guarantees that will be useful for proving Lemma~\ref{Lemma:EdgeDecomposition} and Lemma~\ref{Lemma:CoveringDecomposition}.
First consequence is that all DMGTS obtained this way are consistent specializations.
\begin{lem}\label{Lemma:ObserverConsistentSpecAppendix}
    Let $(\precovering, \charmod)$ be a precovering graph, $\anobserver$ an observer, and $\admgts\in\decompalongof{\precovering, \charmod, \anobserver}$.
    Then, $\admgts$ is a consistent specialization of $\precovering$.
\end{lem}

\begin{proof}
    Let $\admgts=(\openmgts, \charmod)$ be a DMGTS obtained this way.
    We proceed with (1).
    The relations $\inmarkingof{\openmgts}\omegaleq\inmarkingof{\precovering}$ and $\outmarkingof{\openmgts}\omegaleq\outmarkingof{\precovering}$ already hold by definition.
    By definition, for any run $\apath\in\pathsof{\ints}{\openmgts}$, we can remove the observer component from the nodes in the run to get a run in $\precovering$.
    This gives us $\apathp\in\pathsof{\ints}{\openmgts}$ with $\apath\pathequiv\apathp$.
    Now we prove (2).
    Let $\apath\in\interacceptof{\ints}{\restrictto{\omegalequiv{\charmod}}{\rightside}}{\openmgts}$ with $\coordacc{\coordacc{\apath}{\firstindex}}{\rightside}\omegaleq\coordacc{\inmarkingof{\precovering}}{\rightside}$ and $\coordacc{\coordacc{\apath}{\lastindex}}{\rightside}\omegaleq\coordacc{\outmarkingof{\precovering}}{\rightside}$.
    The construction of $\admgts$ ensures that any run $\apath\in\pathsof{\ints}{\admgts}$ with $\coordacc{\coordacc{\apath}{\firstindex}}{\rightside}\omegaleq\coordacc{\inmarkingof{\precovering}}{\rightside}$ already respects the $\rightside$-side of the valuations by extending the consistent assignment $\precovering.\bal$.
    Then, $\apath\in\interacceptof{\ints}{\rightside}{\admgts}$.
\end{proof}

Second consequence allows us to make assuptions about the runs accepted by $\openmgts\in\decompalongof{\precovering, \charmod, \anobserver}$, and find a corresponding run in $\precovering$.
\begin{lem}\label{Lemma:ObserverInformationAppendix}
    Let $(\precovering, \charmod)$ be a precovering graph, $\anobserver$ an observer, and let $\admgts\in\decompalongof{\precovering, \charmod, \anobserver}$.
    If $\apath\in\pathsof{\ints}{\precovering}$ takes the edges $\anedge_{0}\ldots\anedge_{l-1}\in\langof{\anobserver}$, then there is a $\admgts\in\decompalongof{\precovering, \charmod, \anobserver}$ with $\apathp\in\pathsof{\ints}{\admgts}$ and $\apathp\pathequiv\apath$.
\end{lem}

\begin{proof}
    Let $\apath\in\pathsof{\ints}{\precovering}$ take the edges $\anedge_{0}\ldots\anedge_{l-1}\in\langof{\anobserver}$.
    Then, $\anedge_{0}\ldots\anedge_{l-1}$ has an accepting run in $\anobserver$.
    We eliminate (possibly empty) cycles $\apath_{0}, \ldots, \apath_{k}$ on $\astate_{0},\ldots, \astate_{k}$ from this run, such that the resulting $\apathp=\astate_{0}\ldots \astate_{k}$ does not repat states.
    Then $\sigma\in\basicacceptof{\precovering\times\anobserver}$.
    Let the resulting run be $\apathp=\astate_{0}.(\astate_{0}, \anedge_{i_0}, \astate_{1})\ldots \astate_{k}\in\basicacceptof{\precovering\times\anobserver}$.
    Since $\apath_{i}$ is a cycle on $\astate_{i}$ in $\precovering\times\anobserver$ for all $i\leq k$, we can find corresponding runs in $\precovering_{\astate_{i}}^{\anobserver}$.
    Putting these runs together gives us a run $\apath'\in\pathsof{\ints}{\openmgts_{\apathp, \mathsf{raw}}^{\anobserver}}$.
    Since $\openmgts_{\apathp, \mathsf{raw}}^{\anobserver}$ and $\openmgts_{\apathp}^{\anobserver}$ differ only in their valuations, we have $\apath'\in\pathsof{\ints}{\openmgts_{\apathp}^{\anobserver}}$.
\end{proof}

We use Lemma~\ref{Lemma:ObserverInformation} and the construction of the valuations for DMGTS in $\decompalongof{\precovering, \charmod, \anobserver}$ to make the following remark.
\begin{fact}\label{Remark:ObserverLanguageAppendix}
    Let $(\precovering, \charmod)$ be a precovering graph, $\anobserver$ an observer, and let $\admgts\in\decompalongof{\precovering, \charmod, \anobserver}$.
    If $\apath\in\interacceptofshort{\leftside}{\precovering}$ takes the edges $\anedge_{0}\ldots\anedge_{l-1}\in\langof{\anobserver}$, then there is a $\admgts\in\decompalongof{\precovering, \charmod, \anobserver}$ with $\apathp\in\interacceptofshort{\leftside}{\admgts}$ and $\apathp\pathequiv\apath$.
\end{fact}

\subsubsection{Bounded edges, Lemma~\ref{Lemma:EdgeDecomposition}}
We recall the premise of Lemma~\ref{Lemma:EdgeDecomposition}.
It gives us a precovering graph $\precovering$, $\mu\geq 1$, an MGTS context $\acontext{\contextvar}$, a set of counters $\aside\in\set{\leftside, \rightside}$, and an edge $\anedge\in\edgesof{\precovering}$, where $\anedge\not\in\supportof{\sidecharof{\aside}{\acontext{\precovering, \charmod}}}$.
We consider the set of all such edges $\edges\subseteq\edgesof{\precovering}$.
Because $\anedge\not\in\supportof{\sidecharof{\aside}{\acontext{\precovering, \charmod}}}$ for all $\anedge\in\edges'$, the set $A_{\aside}=\setcond{\coordacc{\asol}{\anedge}}{\anedge\in\edges',\;\asol\in\solutionsof{\sidecharof{\aside}{\acontext{\precovering, \charmod}}}}$ is finite, and computable with elementary resources.
In particular, we can calculate $l\in\nat$ with $A_{\aside}\leq l$ with these resources.
In order to fulfill the conclusion of this lemma, we track how many times some $\anedge\in\edges'$ is taken with an observer.
If a run in $\admgts$ takes such an edge at least $l+1$ times in $\precovering$, then we know that it cannot belong to $\interacceptofshort{\aside}{\admgts}$.
This guarantees the infeasibility of $\sidecharof{\aside}{\admgts'}$ for $\admgts'=\acontext{\openmgts, \charmod}$, where the MGTS $\openmgts$ makes sure some $\anedge\in\edges'$ is taken at least $l+1$ times. 
We capture such $(\openmgts, \charmod)$ in $V$.
Note that $\rankless$ is not required to decrease in this case.
We also generate DMGTS that make sure that each $\anedge\in\edges'$ is taken $i_{\anedge}\leq l$ times.
Such DMGTS consist of precovering graphs $\precovering'$ that whose edges are from $\edgesof{\precovering}\setminus\edges'$.
In this case, $\edgesof{\precovering}\setminus\edges'\subseteq\supportof{\sidecharof{\aside}{\admgts}}$ and $\edges'\cap\supportof{\sidecharof{\aside}{\admgts}}=\emptyset$ guarantee $\cyclespaceof{\precovering'}\subset\cyclespaceof{\precovering}$.
This is proven in \cite[Claim 4.7]{Leroux19}.

We proceed with the formal construction of the observer.
$$\anobserver_{\uvvar}=(\set{0, \ldots, l+1}^{\edges'}, \set{0}, \edgesof{\precovering}, \transitions, \finalstates_{\uvvar})$$ 
for $\uvvar\in\set{\ulabel, \vlabel}$, where
\begin{align*}
    \transitions&=\setcond{(x, \anedge', x)}{i\leq l+1, \anedge'\not\in\edges', x\in \set{0, \ldots, l+1}^{\edges'}}\\
    &\cup\setcond{(x, \anedge, y)}{\anedge\in\edges', y[\anedge]=\max(x[\anedge] + 1, l + 1),\\
    &\hspace{5.25em} x[\edges'\setminus\set{\anedge}]=y[\edges'\setminus\set{\anedge}]}
\end{align*}

$\finalstates_{\ulabel}=\set{0, \ldots, l}^{\edges'}$, and $\finalstates_{\vlabel}=\set{0, \ldots, l+1}^{\edges'}\setminus\finalstates_{\ulabel}$.
As we previously hinted at, $\anobserver_{\ulabel}$ and $\anobserver_{\vlabel}$ count how many times some $\anedge\in\edges'$ is taken, with the former accepting values with coordinates below or equal to $l$, and the the latter accepting values with a coordinate above $l$.
We define 
$$U=\decompalongof{\precovering, \charmod, \anobserver_{\ulabel}}\qquad V=\decompalongof{\precovering, \charmod, \anobserver_{\vlabel}}.$$

We proceed with the proof of the first property in Lemma~\ref{Lemma:EdgeDecomposition}.
For any cycle of edges in $\precovering\times\anobserver_{\ulabel}$, we can find a cycle from the edges in $\edgesof{\precovering}\setminus\edges'$.
To see this, we only need to make two observations.
Let $(\astate, x)$ be a state in $\precovering\times\anobserver_{\ulabel}$.
First, since $x[\anedge]\leq l$ for all $\anedge\in\edges'$, taking any transition labeled $\anedge\in\edges'$ from $(\astate, i)$ results in moving to another strongly connected component, as this increases the $\anedge$-count kept by $\anobserver_{\ulabel}$ permanently.
Second, if a transition labeled $\anedge$ is not taken, we can remove the $\anobserver$ component from the nodes to get a cycle made up of the edges in $\edgesof{\precovering}\setminus\edges'$.
We refer to the arguments in the proof of \cite[Claim 4.7]{Leroux19} to obtain $\cyclespaceof{\precovering'}\subset\cyclespaceof{\precovering}$ for all $\openmgts\in U$ and $\precovering'$ in $\openmgts$.
The strict inclusion $\cyclespaceof{\precovering'}\subset\cyclespaceof{\precovering}$ implies that if $\cyclespaceof{\precovering}$ is $i$-dimensional, then $\cyclespaceof{\precovering'}$ is at most $i-1$ dimensional.
So $\coordacc{\rankingof{\precovering}}{d-i}>0$, while $\coordacc{\rankingof{\precovering'}}{d-i'}=0$ for all $i'\leq \sizeof{\leftside\cup\rightside}$ with $i\leq i'$, where $d=\sizeof{\leftside\cup\rightside}$.
Since $\openmgts$ consists of such $\precovering'$, we get $\coordacc{\rankingof{\precovering'}}{d-i'}=0$ for all $i'\leq \sizeof{\leftside\cup\rightside}$ with $i\leq i'$ as well.
We conclude $\rankingof{\openmgts}\rankless(\precovering,\charmod)$.

Now we prove the second property in Lemma~\ref{Lemma:EdgeDecomposition}.
The observers $\anobserver_{\ulabel}$ and $\anobserver_{\vlabel}$ only differ in their final states, the underlying NFA is complete, and $\finalstates_{\ulabel}\cup\finalstates_{\vlabel}=\set{0, \ldots, l+1}^{\edges'}$.
Then, the sequences of edges in any run $\apath\in\interacceptofshort{\leftside}{\precovering, \charmod}$ is accepted in one of $\anobserver_{\ulabel}$ and $\anobserver_{\vlabel}$.
This implies $\apathp\in\interacceptofshort{\leftside}{U\cup V}$ with $\apath\pathequiv\apathp$ by Remark~\ref{Remark:ObserverLanguage}.

Finally, we show the third property.
Let $(\openmgts, \charmod)\in V$.
Towards a contradiction, suppose $\asol\in\solutionsof{\sidecharof{\aside}{\acontext{\openmgts, \charmod}}}$.
We sketch the construction of $\asol'\in\solutionsof{\sidecharof{\aside}{\acontext{\precovering, \charmod}}}$ with $\coordacc{\asol'}{\anedge}\geq l+1$ for some $\anedge\in\edges'$, which contradicts the definition of $A_{\aside}$.
Let $\openmgts=\precovering_{0}.\anupdate_{0}\ldots\anupdate_{r-1}.\precovering_{r}$ for some precovering graphs $\precovering_{0},\ldots, \precovering_{r-1}$ and updates $\anupdate_{0}\ldots\anupdate_{r-1}$ corresponding to edges $\anedge_{0}, \ldots, \anedge_{r-1}$.
As we argued before, any cycle in $\precovering\times\anobserver_{\vlabel}$ (and thus $\precovering_{i}$ for $i\leq r$) has a cycle in $\precovering$ with the same effect on the counters.
Furthermore, the definitions of $\precovering\times\anobserver$ and $\decompalongof{\precovering, \charmod, \anobserver_{\vlabel}}$ ensure that for $\anedge_{0}\ldots\anedge_{r}\in\basicacceptof{\precovering\times\anobserver_{\vlabel}}$, there is a cycle in $\precovering$ with the same effect that takes some $\anedge\in\edges'$ at least $l+1$ times.
Exchanging the values that stem from the edges of $\openmgts$ in $\asol$ by the sum of the Parikh images of these same-effect cycles in $\precovering$, we get $\asol'\in\solutionsof{\sidecharof{\aside}{\acontext{\precovering, \charmod}}}$ with $\coordacc{\asol'}{\anedge}\geq l+1$.
%

\begin{comment}
Then, we have $\apath=\apath_{0}.\apath_{1}.\apath_{2}$ where $\apath_{1}\in\interacceptofshort{\aside}{\openmgts, \charmod}$, and $\apath_{0}.\contextvar.\apath_{2}$ is the part of the run in the outer context $\acontext{\contextvar}$.
%
The construction of $\anobserver_{\vlabel}$, and thus $\openmgts$, guarantees that there is a run $\apathp_{1}\in\pathsof{\ints}{\precovering}$ with $\apathp_{1}\pathequiv\apath_{1}$ and $\coordacc{\parikhof{\apathp_{1}}}{\anedge}\geq l$.
%
Since $(\precovering, \charmod)$ has no intermediary constraints, and by construction $\inmarkingof{\openmgts}=\inmarkingof{\precovering}$ and $\outmarkingof{\openmgts}=\outmarkingof{\precovering}$, we have $\apathp_{1}\in\interacceptofshort{\aside}{\precovering, \charmod}$.
%
Then, $\apath_{0}.\apathp_{1}.\apath_{2}\in\interacceptofshort{\aside}{\acontext{(\precovering, \charmod)}}$.
%
But since $\coordacc{\parikhof{\apathp_{1}}}{\anedge}\geq l$, this implies a solution $\asol\in\solutionsof{\sidecharof{\aside}{\acontext{(\precovering, \charmod)}}}$ with $\coordacc{\asol}{\anedge}\geq l$.
%
This is a contradiction to the definition of $A_{\aside}$ and $A_{\aside}<l$.
\end{comment}

\subsubsection{No covering sequences, Lemma~\ref{Lemma:CoveringDecomposition}}
The premise of Lemma~\ref{Lemma:CoveringDecomposition} yields a precovering graph $\precovering$, $\mu\geq 1$, with $\coveringseqof{}{\precovering, \mu}=\emptyset$ or $\downcoveringseqof{}{\precovering, \mu}=\emptyset$.
We only consider $\coveringseqof{}{\precovering, \mu}=\emptyset$, as $\downcoveringseqof{}{\precovering, \mu}=\emptyset$ can be handled symmetrically.
We will adapt the proof of \cite[Lemma 4.13]{Leroux19}.
However, to be able to apply the arguments in \cite[Lemma 4.13]{Leroux19}, we must deal with the fixed counters of $\precovering$.
In our setting, we define these counters to be those, where no  cycle in $\precovering$ changes the valuation of this counter.
We define the set of counters $\countersp$ to be the fixed counters.
Formally, 
$$J=\setcond{\aplace\in\leftside\cup\rightside}{\text{for all cycles }\aloop\text{ in }\precovering, \coordacc{\effectof{\aloop}}{\aplace}= 0}.$$

For any fixed counter $\aplace\in\countersp$, there is a unique function $\fixedassig{\aplace}:\nodesof{\precovering}\to\ints$, where $\fixedassigof{\aplace}{\precovering.\groot}=\coordacc{\inmarkingof{\precovering}}{\aplace}$, and  $\fixedassigof{\aplace}{\astate}+\coordacc{\effectof{\anedge}}{\aplace}=\fixedassigof{\aplace}{\astatep}$ for all $\astate, \astatep\in\nodesof{\precovering}$ and $\anedge\in\edgesof{\precovering}$ between these states. 
This unique function can be constructed by setting $\fixedassigof{\aplace}{\precovering.\groot}=\coordacc{\inmarkingof{\precovering}}{\aplace}$, and then following the definition of $\fixedassig{\aplace}$ along the edges.
To see that this function is well defined, suppose that we assign two values $c\neq d$ to some $\astate$ by following the sequence of edges $\apath_{c}$ and $\apath_{d}$ from $\fixedassigof{\aplace}{\precovering.\groot}=\coordacc{\inmarkingof{\precovering}}{\aplace}$.
Then, $\coordacc{\effectof{\apath_{c}}}{\aplace}\neq\coordacc{\effectof{\apath_{d}}}{\aplace}$.
Because $\precovering$ is strongly connected, there is a sequence of edges $\apathp$ from $\astate$ back to $\precovering.\groot$.
At least one of $\coordacc{\effectof{\apath_{c}}}{\aplace}\neq-\coordacc{\effectof{\apathp}}{\aplace}$ or $\coordacc{\effectof{\apath_{d}}}{\aplace}\neq-\coordacc{\effectof{\apathp}}{\aplace}$ must hold.
Let wlog. $\coordacc{\effectof{\apath_{c}}}{\aplace}\neq-\coordacc{\effectof{\apathp}}{\aplace}$.
Then, $\apath_{c}$ followed by $\apathp$ is a cycle, with non-zero effect on counter $\aplace$.
This is a contradiction to $j\in\countersp$.

We make a case distinction along the properties of $\countersp$ and $\fixedassig{\aplace}$.
\begin{itemize}
    \item there is a $\aplace\in\countersp$ with $\coordacc{\inmarkingof{\precovering}}{\aplace}\neq\coordacc{\outmarkingof{\precovering}}{\aplace}\in\nat$
    \item there is a $\aplace\in \countersp$ with $\fixedassig{\aplace}:\nodesof{\precovering}\to\nat$
    \item there is $\aplace\in\countersp$ and $\anode\in\nodesof{\precovering}$ with $\fixedassigof{\aplace}{\anode}<0$
    \item  $\countersp\cap\infinitiesof{\precovering}=\emptyset$
\end{itemize}

We proceed with the first case.
Let $\aplace\in\countersp$ with $\coordacc{\inmarkingof{\precovering}}{\aplace}\neq\coordacc{\outmarkingof{\precovering}}{\aplace}$.
This contradicts the feasability of $\sidecharof{\aside}{\precovering, \charmod}$, where $\aplace\in\aside$.
The reason is that any solution to $\sidecharof{\aside}{\precovering, \charmod}$ implies a union of loops in $\precovering$ with the effect $\coordacc{\outmarkingof{\precovering}}{\aplace}-\coordacc{\inmarkingof{\precovering}}{\aplace}$ on $\aplace$, but loops have $0$ effect on $\aplace$ by the definition of $\countersp$.

For the next case, let there be $\aplace\in \countersp$ with $\fixedassig{\aplace}:\nodesof{\precovering}\to\nat$.
Then, we modify consistent-assignment and the final valuation in $\precovering$ to get $\precovering'= (\precovering.\avas, (\precovering.\groot, \inmarkingof{\precovering}), (\precovering.\groot, z), \phi_{\aplace})$.
We define the assignment by $\coordacc{\phi_{\aplace}(\anode)}{\aplacep}=\coordacc{\phi(\anode)}{\aplacep}$ and $\coordacc{\phi_{\aplace}(\anode)}{\aplace}=\fixedassigof{\aplace}{\anode}$ for all $\aplacep\in\leftside\cup\rightside\setminus\set{\aplace}$, $\anode\in\nodesof{\precovering}$.
For the final valuation, we let $\coordacc{z}{\aplacep}=\coordacc{\outmarkingof{\precovering}}{\aplacep}$ for all $\aplacep\in\leftside\cup\rightside\setminus\set{\aplace}$, and $\coordacc{z}{\aplace}=\coordacc{\outmarkingof{\precovering}}{\aplace}$ if $\coordacc{\outmarkingof{\precovering}}{\aplace}\in\nat$, and $\coordacc{z}{\aplace}=\phi_{j}(\precovering.\groot)$.
We modify the final valuation, in order to meet the definition of a precovering graph.
This satisfies the requirements for a consistent assignment.
Furthermore, we have $\infinitiesof{\inmarkingof{\precovering'}}+\infinitiesof{\outmarkingof{\precovering'}}+\infinitiesof{\precovering'}<\infinitiesof{\inmarkingof{\precovering}}+\infinitiesof{\outmarkingof{\precovering}}+\infinitiesof{\precovering}$ and $\edgesof{\precovering}=\edgesof{\precovering'}$.
This yields $(\precovering', \charmod)\rankless(\precovering, \charmod)$.
To see that $(\precovering', \charmod)$ is a consistent specialization, consider that we only made valuations stricter.
So, any $\apath\in\pathsof{\ints}{\precovering', \charmod}$ with $\coordacc{\coordacc{\apath}{\firstindex}}{\rightside}\omegaleq\coordacc{\inmarkingof{\precovering'}}{\rightside}$ and $\coordacc{\coordacc{\apath}{\lastindex}}{\rightside}\omegaleq\coordacc{\outmarkingof{\precovering'}}{\rightside}$, we have $\apath\in\interacceptof{\ints}{\rightside}{\precovering', \charmod}$ since $\precovering'$ is a precovering graph.
This, along with the fact that we did not introduce any new runs, fulfill both conditions of consistent specialization.
So $U=\set{(\precovering', \charmod)}$ and $V=\emptyset$ satisfy all properties of Lemma~\ref{Lemma:DecoupledDecomposition}.

The remaining two cases are those where an actual decomposition takes place.
Let the largest transition effect in $\precovering$ be $l$.
Let $B=(\sizeof{\nodesof{\precovering}}\cdot l\cdot C)^{\sizeof{\countersp}+1!}$ and $C=\max(\setcond{\coordacc{\inmarkingof{\precovering}}{\aplacep}}{\aplacep\in\leftside\cup\rightside}\setminus\set{\omega})+1$.
We construct the observer 
$$\anobserver_{\aplace, \uvvar}=(\set{\bot, 0, \ldots, B-1, \omega}, \set{\coordacc{\inmarkingof{\precovering}}{\aplace}}, \edgesof{\precovering}, \transitions_{\aplace}, \finalstates_{\aplace, \uvvar})$$
for all $\aplace\in\leftside\cup\rightside$ and $\uvvar\in\set{\ulabel, \vlabel}$.
The transitions
\begin{align*}
    \transitions_{\aplace}=&\setcond{(i, \anedge, i')}{0\leq i, i'<B, \anedge\in\edgesof{\precovering}, i'=i+\coordacc{\effectof{\anedge}}{\aplace}}\;\cup\\
    &\setcond{(i, \anedge, \bot)}{0\leq i < B, i+\coordacc{\effectof{\anedge}}{\aplace}<0}\;\cup\\
    &\setcond{(i, \anedge, \omega)}{0\leq i < B, i+\coordacc{\effectof{\anedge}}{\aplace}\geq B}\;\cup\\
    &\setcond{(\bot, \anedge, \bot), (\omega, \anedge, \omega)}{\anedge\in\edgesof{\precovering}}
\end{align*}
track the counter $\aplace$ from $\coordacc{\inmarkingof{\precovering}}{\aplace}$, as long as its value is positive and below $B$.
The final states $\finalstates_{\aplace,\uvvar}$
\begin{align*}
    \finalstates_{\aplace,\ulabel}&=\setcond{0\leq i<B}{i\omegaleq \coordacc{\outmarkingof{\precovering}}{\aplace}}\;&\text{for all }\aplace\in\leftside\cup\rightside\setminus\infinitiesof{\inmarkingof{\precovering}}\\
    \finalstates_{\aplace, \vlabel}&=\set{0, \ldots, B-1, \bot}\setminus\finalstates_{\aplace, \ulabel}\qquad&\text{for all }\aplace\in\rightside\setminus\infinitiesof{\inmarkingof{\precovering}}\\
    \finalstates_{\aplace, \vlabel}&=\emptyset\qquad&\text{for all }\aplace\in\leftside\cup\infinitiesof{\inmarkingof{\precovering}}.
\end{align*}
are defined to capture runs from $\interacceptofshort{\leftside}{\precovering, \charmod}$ by counting up to bound.
The final states where $\uvvar=\ulabel$ accept the runs whose edges would reach $\coordacc{\outmarkingof{\precovering}}{\aplace}$ from $\coordacc{\inmarkingof{\precovering}}{\aplace}$ on the counter $\aplace$ without exceeding the bound $B$.
For $\uvvar=\vlabel$, the final states track the violation of the constraints in $\precovering$.
We only need to track the runs that violate constraints on $\rightside$ counters, as those that violate $\leftside$ counters were not in $\interacceptofshort{\leftside}{\precovering, \charmod}$ in the first place.
We do not track any runs if $\aplace$ is initially $\omega$.
We will argue that we do not miss any $\interacceptofshort{\leftside}{\precovering, \charmod}$ runs as follows.
If a $\interacceptofshort{\leftside}{\precovering, \charmod}$ run were to escape $\finalstates_{\aplace, \ulabel}$ for all $\aplace\in\aplace\in\leftside\cup\rightside\setminus\infinitiesof{\inmarkingof{\precovering}}$, and $\finalstates_{\aplace, \vlabel}$ for all $\aplace\in\aplace\in\rightside\setminus\infinitiesof{\inmarkingof{\precovering}}$, then its non-fixed counters must be pumpable by Lemma~\ref{Lemma:Rackoffesque}.
This contradicts $\coveringseqof{}{\precovering, \charmod}=\emptyset$.

For both of the remaining cases, we define $V$ the same way 
$$V=\bigcup_{\aplace\in\infinitiesof{\precovering}}\decompalongof{\precovering, \charmod, \anobserver_{\aplace, \vlabel}}.$$
Since the last property of Lemma~\ref{Lemma:DecoupledDecomposition} only concerns $V$, we handle this property by the same proof in both cases.

We show that for all $\admgts\in V$, $\rightcharof{\admgts}$ is infeasible.
Suppose that there is an $\admgts=(\openmgts, \charmod)\in V$, such that $\rightcharof{\admgts}$ is feasible.
Let $\aplace\in\infinitiesof{\precovering}$ with $\admgts\in\decompalongof{\precovering, \charmod, \anobserver_{\aplace, \vlabel}}$.
This implies $\aplace\in\rightside$.
Let $\asol\in\solutionsof{\rightcharof{\admgts}}$.
We obtain $\asol'$ from $\asol$ by fixing $\coordacc{\asol'}{\precovering'', \mathsf{in}, \aplace}=\coordacc{\asol}{\precovering'', \mathsf{in}, \aplace}=\coordacc{\inmarkingof{\precovering}}{\aplace}$ and removing all edge applications along with their effects on the remaining variables that represent counter values.
We show that properties of $\asol'$ and $\openmgts$ imply that $\asol$ is not a solution.
We make a case distinction along the form of $\openmgts$.
For the sake of brevity, let $\precoveringp_{(\astate, i)}=\precovering_{(\astate, i)}^{\anobserver_{\aplace, \vlabel}}$ for all $\astate\in\nodesof{\precovering}$ and $i\in\set{\bot, 0, \ldots, B, \omega}$.
For the first case, we have some $\astate_{0}, \ldots, \astate_{r}$ and $i_{0}, \ldots, i_{r-1}\in\set{0, \ldots, B-1}$, where
$$\openmgts=\precoveringp_{(\astate_{0}, i_{0})}\ldots\precoveringp_{(\astate_{r-1}, i_{r-1})}\anupdate_{r-1}\precoveringp_{(\astate_{r}, \bot)}\ldots$$
For the second case, we have some $\astate_{0}, \ldots, \astate_{k}$ and $i_{0}, \ldots, i_{k}\in\set{0, \ldots, B-1}$ with $i_{k}\neq\outmarkingof{\precovering}\in\nat$ and
$$\openmgts=\precoveringp_{(\astate_{0}, i_{0})}.\anupdate_{0}\ldots\anupdate_{k-1}\precoveringp_{(\astate_{k}, i_{k})}.$$

We proceed with the first case.
The states of $\anobserver_{\aplace, \vlabel}$ track the counter $\aplace$ precisely up to $B-1$.
So a run starting with a valuation $\coordacc{\inmarkingof{\precovering}}{\aplace}$ on counter $\aplace$ and following application of the edges $\anedge_{0}\ldots\anedge_{r-1}$, that correspond to $\anupdate_{0}\ldots\anupdate_{r-1}$, reaches a negative counter valuation.
Since these are the only edges that effect the counters in $\asol'$ and $\coordacc{\asol'}{\precoveringp_{(\astate_0, i_0)}, \mathsf{in}, \aplace}=\coordacc{\inmarkingof{\precovering}}{\aplace}$,
we know that $\coordacc{\asol'}{\precoveringp_{(\astate_{r}, \bot)}, \mathsf{in}, \aplace}<0$.
We argue that $\coordacc{\asol}{\precoveringp_{(\astate_{r}, \bot)}, \mathsf{in}, \aplace}<0$ must also hold.
Since $\anobserver_{\aplace, \vlabel}$ tracks the $\aplace$ counters precisely, and therefore any cycle from $i$ to $i$ with $i< B$ and $0\leq i$ in $\anobserver_{\aplace, \vlabel}$ with $i\in\set{0, \ldots, B-1}$ is guaranteed to have $0$ effect.
Then, a cycle $\aloop$ in any of the precovering graphs $\precoveringp_{(\astate_{0}, i_{0})}, \ldots, \precoveringp_{(\astate_{r-1}, i_{r-1})}$ has $\coordacc{\effectof{\aloop}}{\aplace}=0$.
So removing the effects of these cycles from $\asol$ does not change the value of $\coordacc{\asol}{\precoveringp_{(p_r, \bot)}, \mathsf{in}, \aplace}$.
This gives us $\coordacc{\asol}{\precoveringp_{(p_r, \bot)}, \mathsf{in}, \aplace}=\coordacc{\asol'}{\precoveringp_{(p_r, \bot)}, \mathsf{in}, \aplace}<0$, which contradicts $\asol\in\solutionsof{\rightcharof{\admgts}}$.

For the second case, we apply the same argument and observe that a cycle $\aloop$ in any precovering graph of $\openmgts$ has $\coordacc{\effectof{\aloop}}{\aplace}=0$.
Then, we have $\coordacc{\asol}{\precoveringp_{(p_r, \bot)}, \mathsf{in}, \aplace}=\coordacc{\asol'}{\precoveringp_{(p_r, \bot)}, \mathsf{in}, \aplace}\neq\coordacc{\outmarkingof{\precovering}}{\aplace}\in\nat$.
This also contradicts $\asol\in\solutionsof{\rightcharof{\admgts}}$.

Now we handle the construction of $U$ and the remaining properties for the first case.
Let $\aplace\in\countersp$ and $\anode\in\nodesof{\precovering}$ with $\fixedassigof{\aplace}{\anode}<0$.
Because $\precovering$ is strongly connected, there is an ingoing edge $\anedge=(\anode', \aletter, x, \anode)\in\edgesof{\precovering}$ for some $\anode'$, $\aletter$, and $x$.
We remove $\anedge$ from $\precovering$ as follows.
We construct $\precovering'$ from $\precovering$ by removing $\anedge$, along with all $\anodep\in\nodesof{\precovering}$ that are not in the same strongly connected component as $\precovering.\groot$ after the removal of $\anedge$.
The result is strongly connected, and we let $U=\set{\precovering'}$.

Towards a proof of the second property of Lemma~\ref{Lemma:EdgeDecomposition}, we show that $V$ captures all $\leftside$-accepting runs in $\precovering$ that take $\anedge$.
If $\aplace\in\leftside$, then any run that is $\leftside$-accepted cannot take $\anedge$: since an $\leftside$-accepted a run starts from $\fixedassigof{\aplace}{\groot}=\coordacc{\inmarkingof{\precovering}}{\aplace}$, it must reach $\anode$ with $\fixedassigof{\aplace}{\anode}<0$ upon taking $\anedge$, which contradicts the positivity requirement of $\interacceptofshort{\leftside}{\precovering, \charmod}$.
If $\aplace\in\rightside$, let $\apath\in\interacceptofshort{\leftside}{\precovering, \charmod}$ take $\anedge$.
Then, some prefix $\apath'$ of $\apath$ must have an effect $u$ on counter $j$, such that $\coordacc{\outmarkingof{\precovering}}{\aplace}+u<0$.
This is required by $\fixedassig{\aplace}$.
We know that $\apath'$ cannot have a prefix that has an effect $u'$ on $\aplace$ with $\coordacc{\outmarkingof{\precovering}}{\aplace}+u'\geq B$.
We know this, because $\fixedassig{\aplace}(\anode)$ can be at most $l\cdot \sizeof{\nodesof{\precovering}}$ larger than $\coordacc{\inmarkingof{\precovering}}{\aplace}$ and $B\geq  \sizeof{\nodesof{\precovering}}\cdot l\cdot \coordacc{\inmarkingof{\precovering}}{\aplace}$ is guaranteed by the construction.
Thanks to boundedness, the edges of $\apath$ have a run in $\anobserver_{\aplace, \vlabel}$ that reaces $\bot$.
By Remark~\ref{Remark:ObserverLanguage} there is $\apathp\in\interacceptofshort{\leftside}{\openmgts}$ for some $\openmgts\in\decompalongof{\precovering, \charmod, \anobserver_{\aplace, \vlabel}}$ with $\apathp\pathequiv\apath$.
Since $V$ captures all $\leftside$-accepting runs that use $\anedge$, all remaining runs must avoid $\anedge$.
Furthermore, because $\leftside$-accepting, uncaptured runs in $\precovering$ are cycles on $\precovering.\groot$, they cannot visit the removed nodes.
So, for all $\apath\in\interacceptofshort{\leftside}{\precovering, \charmod}$, there is a $\apathp\in\interacceptofshort{\leftside}{U\cup V}$ with $\apath\pathequiv\apathp$.
Now we show the first property of Lemma~\ref{Lemma:EdgeDecomposition}, $\rankingof{\precovering'}<_{\mathsf{lex}}\rankingof{\precovering}$.
It suffices to observe $\edgesof{\precovering'}\subset\edgesof{\precovering}$, since this also implies $\cyclespaceof{\precovering'}\subseteq\cyclespaceof{\precovering}$.
The argument for consistent specialization is the same as the one we gave in the case with $\aplace\in\countersp$ and $\fixedassig{\aplace}:\nodesof{\precovering}\to\nat$.

Finally we the last case.
Let $\infinitiesof{\precovering}\cap\countersp=\emptyset$ hold.
We let 
$$U=\bigcup_{\aplace\in\infinitiesof{\precovering}}\decompalongof{\precovering, \charmod, \anobserver_{\aplace, \ulabel}}.$$
We proceed with the first property of Lemma~\ref{Lemma:CoveringDecomposition}, and show $\openmgts\rankless\precovering$ for all $(\openmgts, \charmod)\in U$.
Let $\cyclespaceof{\precovering}$ be $d$ dimensional, $D=\sizeof{\leftside\cup\rightside}$, and $(\openmgts, \charmod)\in\decompalongof{\precovering, \charmod, \anobserver_{\aplace, \ulabel}}$ for some $\aplace\in\infinitiesof{\precovering}$.
Then, $\coordacc{\rankingof{\precovering}}{D-d}>0$.
We argue that for all precovering graphs $\precovering'$ in $\openmgts$, $\cyclespaceof{\precovering'}\subset\cyclespaceof{\precovering}$ holds.
This shows $(\openmgts, \charmod)\rankless(\precovering, \charmod)$, similarly to the proof of Lemma~\ref{Lemma:EdgeDecomposition}.
As in the previous case, we know that $\openmgts$ can neither contain $\precoveringp_{(\astate, \bot)}$ nor $\precoveringp_{(\astate, \omega)}$ for some $\astate\in\nodesof{\precovering}$ by the definition of $\finalstates_{\aplace, \ulabel}$.
So we only need to show the strict inclusion $\cyclespaceof{\precoveringp_{(\astate, i)}}\subset\cyclespaceof{\precovering}$
for $\astate\in\nodesof{\precovering}$ and $i<B$ with $0\leq i$.
The inclusion $\cyclespaceof{\precoveringp_{(\astate, i)}}\subseteq\cyclespaceof{\precovering}$ is clear, since for each loop in $\cyclespaceof{\precoveringp_{(\astate, i)}}$, there is one in $\precovering$ with the same effect.
Now suppose $\cyclespaceof{\precoveringp_{(\astate, i)}}=\cyclespaceof{\precovering}$.
We know that $\aplace\in\infinitiesof{\precovering}$ and $\infinitiesof{\precovering}\cap\countersp=\emptyset$, so $\aplace\not\in\countersp$, i.e. $\aplace$ is not fixed.
Then, there is a cycle $\aloop$ in $\precovering$ with $\coordacc{\effectof{\aloop}}{\aplace}\neq 0$.
This means $\effectof{\aloop}\in\cyclespaceof{\precovering}$.
Because of the supposed equality, $\effectof{\aloop}\in\cyclespaceof{\precoveringp_{(\astate, i)}}$ must hold.
Then, $\coordacc{\effectof{\aloop}}{\aplace}$ must be a linear combination of cycle effects $\coordacc{\effectof{\aloop_{0}}}{\aplace},\ldots, \coordacc{\effectof{\aloop_{r}}}{\aplace}$ in $\precoveringp_{(\astate, i)}$.
This implies that there is a cycle effect $\coordacc{\effectof{\aloop_{i}}}{\aplace}\neq 0$.
Because $\anobserver$ concretely tracks the value of $\aplace$, all cycles $\aloop'$ in $\precoveringp_{(\astate, i)}$ must have $\coordacc{\effectof{\aloop'}}{\aplace}=0$.
This is a contradiction.

Finally, we show the second property of Lemma~\ref{Lemma:CoveringDecomposition}.
Let $\apath'=(\astate_{0}, \aconf_{0}').\anedge_{0}\ldots\anedge_{r-1}.(\astate_{r}, \aconf_{r}')\in\interacceptofshort{\leftside}{\precovering, \charmod}$.
Further let $\apath=(\astate_{0}, \aconf_{0}).\anedge_{0}\ldots\anedge_{r-1}.(\astate_{r}, \aconf_{r})$ where the $\rightside$ counter valuations have been translated such that $\coordacc{\aconf_{0}}{\rightside}\omegaleq\coordacc{\inmarkingof{\precovering}}{\rightside}$ holds as well.
We must show the existence of $\apathp\in\interacceptofshort{\leftside}{U\cup V}$ with $\apathp\pathequiv\apath$.
By Remark~\ref{Remark:ObserverLanguage}, this is implied by $\anedge_{0}\ldots\anedge_{r-1}$ having an accepted run in $\anobserver_{\aplace,\uvvar}$ for some $\aplace\in\infinitiesof{\precovering}$ and $\uvvar\in\set{\ulabel, \vlabel}$.
We reason with a contradiction.
Suppose for each $\aplace\in\infinitiesof{\precovering}$, there is a $m\leq r$ with $\coordacc{\aconf_{m}}{\aplace}\geq B$, and $\coordacc{\aconf_{m'}}{\aplace}\geq 0$ for all $m'\leq m$.
Then, Lemma~\ref{Lemma:Rackoffesque} applies to show that there is a $\apathp\in\pathsof{\infinitiesof{\precovering}}{\precovering}$ with $\coordacc{\apathp}{0}=(\precovering.\groot, \aconf_{0})$, $\aconf_{0}\omegaleq\inmarkingof{\precovering}$, and $\coordacc{\apathp}{\lastindex}=(\precovering.\groot, x')$ with $\coordacc{x'}{\aplace}\geq C >\max(\setcond{\coordacc{\inmarkingof{\precovering}}{\aplacep}}{\aplacep\in\leftside\cup\rightside}\setminus\set{\omega})$.
We argue that $\apathp\in\coveringseqof{}{\precovering}$.
Membership to $\coveringseqof{}{\precovering}$ does not impose any restrictions on counters $\aplace\in\infinitiesof{\inmarkingof{\precovering}}$.
The argument for the counters $\aplace\in\infinitiesof{\precovering}\setminus\infinitiesof{\inmarkingof{\precovering}}$ is clear from the properties delivered by Lemma~\ref{Lemma:Rackoffesque}.
The counters $\aplace\not\in\infinitiesof{\precovering}$, are already tracked by $\precovering.\varphi$.
Then, these counters can neither become negative nor have $\coordacc{x'}{\aplace}\neq\coordacc{\inmarkingof{\precovering}}{\aplace}$.
This concludes the proof.

\section{Appendix: Complexity} 
\subsection{Lower Bound}
\begin{lem}
    \textsf{$\nat$-REGSEP} is $\mathbb{F}_{\omega}$-hard, even if the input languages are promised to be disjoint and the only separator candidate is $\emptyset$. 
\end{lem}
\begin{proof}
    We show how to reduce the reachability problem for VASS. 
    Assume we are given the VASS~$\avasp$ for which we should check reachability. 
    There are VASS $\avasp'$ and $\avasp''$ whose languages are disjoint, $\speclangof{\nat}{\avasp'}\cap\speclangof{\nat}{\avasp''}=\emptyset$, but where regular separability fails, $\speclangof{\nat}{\avasp'}\mathop{\not\hspace{-0.05cm}|}\speclangof{\nat}{\avasp''}$. 
    Let 
    $\avasp=(\avas, (\instate, \incounters), (\outstate, \outcounters))$ 
    and $\avasp'=(\avas', (\instate', \incounters'), (\outstate', \outcounters'))$. 
    Assume wlog. that the sets of states resp. counters in $\avasp$ and $\avasp'$ are disjoint. 
    We define the VASS
    \begin{align*}
        \avas_{\mathit{new}}\ =\ \avas_{\epsilon}\uplus\set{\anedge_{\mathit{new}}}\uplus \avas'\ . 
    \end{align*}
    It first executes a version of $\avas$ where all edges are labeled by~$\varepsilon$ and then moves to $\avas'$ using the new edge $\anedge_{\mathit{new}}=(\outstate, \anupdate, \instate')$. 
    The update removes the final counter valuation $\outcounters$ from the counters in $\avas$, and adds the counter valuation $\incounters'$ to the counters in $\avas'$,  $\actionbalof{\anupdate}=(-\outcounters, \zerovec)+(\zerovec, \incounters')$. 
    The labeling is $\lambda(\anupdate)=\varepsilon$. 
    We define $\avasp_{\mathit{new}}=(\avas_{\mathit{new}}, (\instate, (\incounters, \zerovec)), (\outstate', (\zerovec, \outcounters')))$ and claim that 
    \begin{alignat*}{5}
        \acceptof{\nat}{\omegaleq}{\avas}&\neq \emptyset\quad&\text{implies}\quad \speclangof{\nat}{\avasp_{\mathit{new}}} &= \speclangof{\nat}{\avasp'}\\
        \acceptof{\nat}{\omegaleq}{\avas}&= \emptyset\quad&\text{implies}\quad \speclangof{\nat}{\avasp_{\mathit{new}}} &= \emptyset\ .
    \end{alignat*}
        As a consequence, reachability in $\avas$ fails, $\acceptof{\nat}{\omegaleq}{\avas}= \emptyset$,  if and only if $\speclangof{\nat}{\avasp_{\mathit{new}}}$ and $\speclangof{\nat}{\avasp''}$ are separable $\emptyset$, which is a regular language. 
        The reduction can be computed in logarithmic space. 
\end{proof}
