# Supplementary material for: On the Separability Problem of VASS Reachability Languages
Source: arXiv:2401.16095 source file (2026-11-16)
Supplement: Supplementary file 4 [file appendix_dmgts.tex]

\section{Appendix: DMGTS}
\begin{proof}[Proof of Lemma~\ref{Lemma:EasyInclusion}]
    Let $\aword\in\rightlangof{\admgts}$.
    Then there is a run $\arun$ in~$\admgts$ labeled by $\edgelabelof{\apath}=\aword$ that remains non-negative and that is accepting on $\rightside$. 
    By the definition of DMGTS, the effects of letters on the counters in $\rightside$ agree with the effects that these letters have in the VASS $\dyckvas_{\dyckdims}$.
    This allows us to construct a run $\apath'\in\acceptof{\nat}{\omegaleq}{\dyckvas_{\dyckdims}}$ that has the same counter valuations and updates. 
    Hence, we have $\aword\in \dycklangn{\dyckdims}$. 
\end{proof}
